# Supplementary material for: Critical coupling to Tamm plasmons
Source: arXiv:1411.0608 source file (2014-11-03)
Supplement: Supplementary file 1 [file SI.pdf]

# *Supplementary Information for:* Critical coupling to Tamm plasmons

Baptiste Auguié*, Axel Bruchhausen, and Alejandro Fainstein

*Centro Atómico Bariloche e Instituto Balseiro, S.C. de Bariloche, Río Negro 8400, Argentina*

November 3, 2014

## 1 Drude model

The dielectric function of gold was obtained from Johnson and Christy [1], with the exception of Fig. 4(f) of the main manuscript where we varied the intrinsic loss in the metal with a Drude model of the form,

$$\varepsilon = \varepsilon_\infty - \frac{\omega_p^2}{\omega^2 + i\omega\gamma}. \tag{1}$$

The plasma frequency $\omega_p = 1.332 \times 10^{16}\,\mathrm{rad\,s^{-1}}$ and the background dielectric constant $\varepsilon_\infty = 7.91$ were kept constant, while the electron scattering rate $\gamma$ was varied around the best-fit value of $1.11 \times 10^{14}$ Hz as shown in Fig. S1.

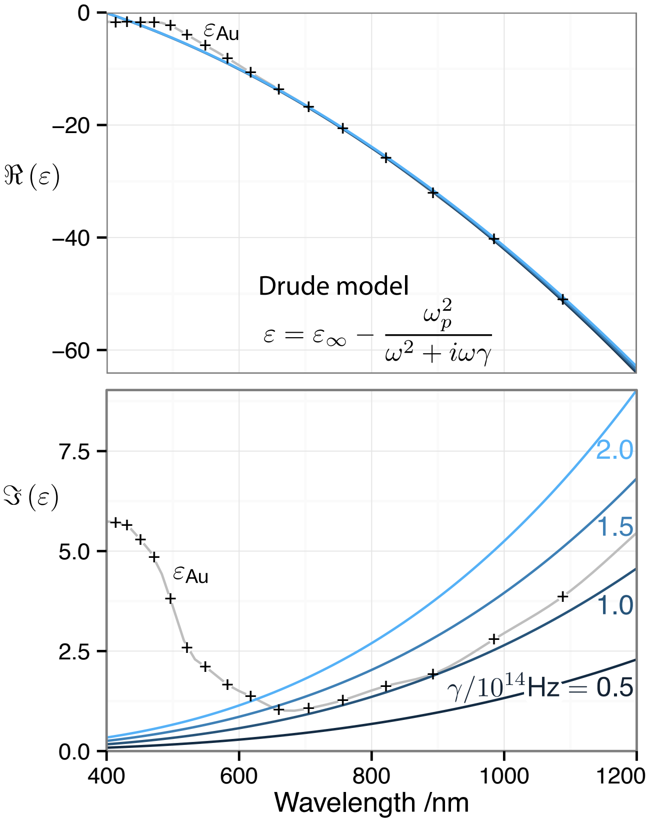


**Figure S1.** Dielectric function of gold in the visible–near-IR region, divided in real and imaginary parts (top and bottom panels, respectively). Data points are from Johnson and Christy [1], connected with a smoothing spline. The blue curves present for comparison the dielectric function of a Drude model given by the equation, with different values of the electron scattering rate $\gamma$.

## 2 Field profile inside the DBR

The Tamm mode is confined between two mirrors – the metal layer on one side, and the DBR on the other. In this sense, it is perhaps more similar to a cavity mode than to surface plasmon-polaritons excited via attenuated total internal reflection. Figure S2 presents the mode profile inside the structure at resonance, and compares the field intensity distribution to a single DBR mirror. Although the magnitude is very different, due to the resonant excitation of TPs, the modal field closely follows the characteristic decay of light reflected off a DBR, with an exponential decay envelope dictated by the refractive index contrast between layers, and a periodic modulation.

*baptiste.auguie@cab.cnea.gov.ar

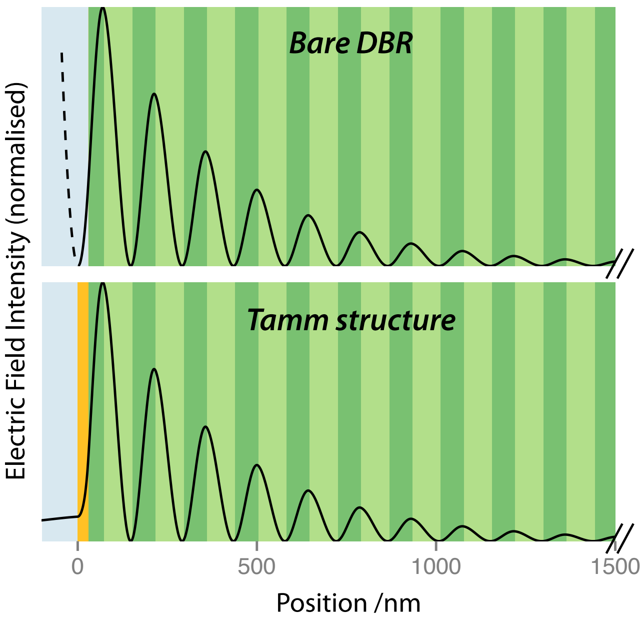


**Figure S2.** Spatial distribution of the electric field intensity $|E|^2$ inside the DBR for a bare DBR (no metal coating), and a Tamm structure. The wavelength for both simulations is 965 nm, corresponding to the Tamm plasmon resonance of the bottom structure, which consists of 50 DBR pairs and a 30 nm thick Au film, illuminated from the air-Au side (the absorbance reaches unity).

Figure S3 illustrates the effect of the spacer thickness on the spatial distribution of the electric field associated with TPs, for both directions of incidence corresponding to Fig. 5 of the main manuscript. We note the following characteristics:

- The exponential envelope of the field presents a stronger decay when the resonance frequency approaches the centre of the DBR stopband. This is an expected feature for a defect mode in a photonic crystal, more strongly localised near the centre of the stopband [2].

- The phase of the field oscillations *relative to the metal–DBR interface* is remarkably insensitive to small variations of spacer thickness. This holds true for uncoated DBRs illuminated from the air side (not shown), and can be understood as a characteristic feature of the evanescent Bloch wave within the DBR for frequencies inside the photonic stop band.

- The intensity of the Tamm mode inside the Au layer is independent of spacer thickness for the second configuration (incidence from air), except for positive values of $\delta s$ (spacer thicker than its nominal value of $\lambda/4$) which bring the Tamm plasmon resonance close to the red side of the stopband. This constant field is expected from the far-field spectra shown in Fig. 5 of the main manuscript, as the absorbance of the structure is proportional to the integrated electric field intensity inside the metal layer. In contrast, the case of incidence from the substrate-DBR side shows a marked variation of field intensity near the Au layer, which we can directly relate to the destruction of critical coupling with any spacer thickness variation.

## 3 Tamm plasmon dispersion

The condition of normal incidence was chosen in the main manuscript to simplify the discussion and focus on the asymmetric response and critical coupling conditions. A defining feature of Tamm plasmons is the possibility of excitation within the light cone, that is, with freely-propagating incident light. In this sense, the case of normal incidence is of particular relevance for practical applications. It is clear however that the angular dispersion of the mode also brings new interesting features, and even richer physics [3]. Although a comprehensive study of critical coupling at arbitrary incidence angle is beyond the scope of the present study, we provide further data at oblique incidence in Figs. S4, S5 for completeness, to see the deterioration of critical coupling for two configurations optimised at normal incidence.

Figure S4 presents the map of absorbance for the Tamm mode as a function of incident angle, from 0 degrees to 50 degrees in the semi-infinite GaAs substrate. Tamm modes with TE and TM polarisation present a different dispersion, and both cases are treated separately. With an increase in incidence angle, the normal component of the wavevector decreases, resulting in a progressive shift of the stopband, and Tamm mode, which all appear as parabolic arcs in the figure. The maximum absorbance at the TP resonance remains relatively high up to $\sim 20°$, after which the absorbance drops pro-

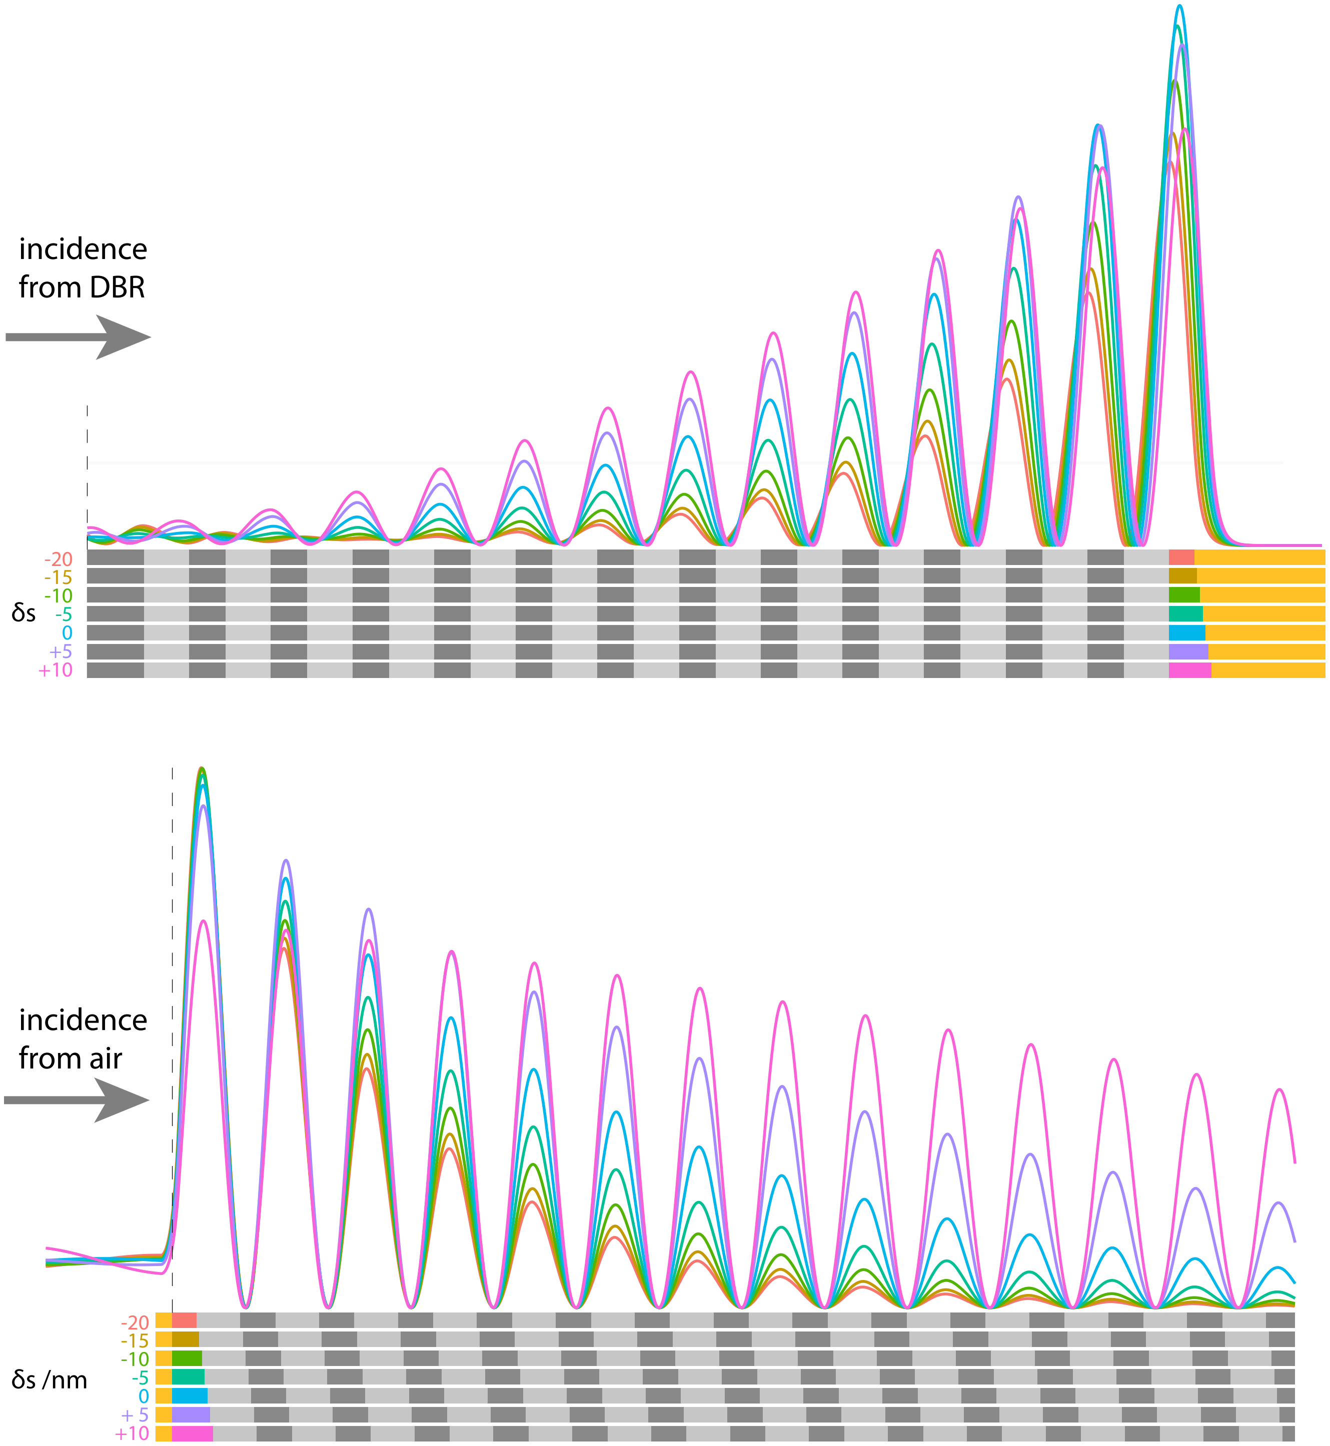


**Figure S3.** Profile of the electric field intensity inside a Tamm structure, with varying spacer thickness. (Top) Incidence from the substrate–DBR side on a structure with 13 DBR pairs and an optically thick Au layer. The thickness variation $\delta s$ ranges from $-20$ nm to $+10$ nm around the nominal value $\lambda/4 = 64.2$ nm. The structures are aligned with the first interface reached by the incident light, therefore the variation in spacer thickness translates into a shift of the metal interface at the other end. The field profiles are colour-coded with the corresponding structure. (Bottom) Light is incident from the air side onto a 30 nm thick Au layer followed by 35 pairs of DBR layers. The structures with varying spacer thickness are aligned against the air–Au interface.

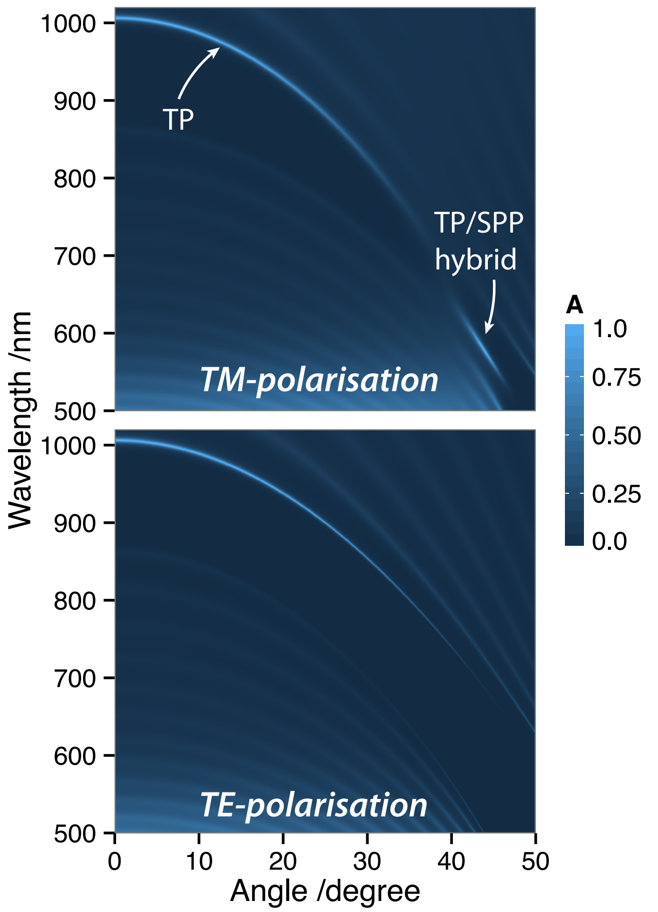


**Figure S4.** Angular dispersion of the Tamm mode, illuminated from the substate-DBR side. The structure is that of Fig. 4 (a) of the main manuscript, i.e. a finite DBR of 13 pairs followed by an optically thick gold film. The angle of incidence with respect to the normal is taken within the semi-infinite substrate. Top and bottom panels correspond to TM- and TE- polarisations, respectively.

gressively and disappears after about $\sim 50°$.

Interestingly, TM-polarisation allows coupling (anti-crossing) between the Tamm mode and propagating surface plasmon-polaritons on the opposite side of the metal film; this new hybrid mode was previously studied and holds promise for surface-enhanced spectroscopies [4, 5]. Absorption may reach unity for optimum coupling conditions (thickness of the metal layer, here 30 nm). Is it important to note that in those simulations, we considered the DBR materials to be non-absorbing dielectrics with a constant refractive index. This is not the case of GaAs (and to a minor extent AlAs), which sustain considerable absorption in the visible region. The lower part of these dispersion maps (below about 700 nm) should therefore apply only to other materials with a transparency window in the visible region.

A broad and omnidirectional absorption spectrum is beneficial in several applications of perfect absorbers such as solar cells [6]. The results of Fig. S4 suggest that this configuration is more suitable to narrow-band and directional applications. However, we should note that the incident angle is defined in the substrate (of high refractive index). The reverse structure, where light is incident from the air-Au side, is perhaps more suitable for omni-directional applications. The results for this configuration are shown in Fig. S5. First, we note a much more limited spectral shift of the TP across the entire 0°–90° angular range accessible from the air side. The range of incident in-plane wavevectors is substantially reduced with incidence from the low-index side, the same effect that allows an apparent photonic bandgap for one-dimensional photonic crystals with sufficient index contrast [2].

A strong absorbance is maintained up to $\sim 60°$ for both polarisations. However, a different behaviour is observed approaching grazing incidence, as the normal and tangential components of the fields for both polarisations must conform to different boundary conditions at the air-metal interface.

## References

[1] P. B. Johnson and R. W. Christy. Optical constants of noble metals. *Phys. Rev. B*, 6:4370–4379, 1972.

[2] J. D. Joannopoulos, R. D. Meade, and J. N. Winn. *Photonic Crystals: Molding the Flow of Light*. Princeton University Press, Singapore, 1995.

[3] Andreas Tittl, Moshe G. Harats, Ramon Walter, Xinghui Yin, Martin Schäferling, Na Liu, Ronen Rapaport, and Harald Giessen. Quantitative angle-resolved small-spot reflectance measurements on plasmonic perfect absorbers: Impedance matching and disorder effects. *ACS Nano*, 2014.

[4] B. I. Afinogenov, V. O. Bessonov, A. A. Nikulin, and A. A. Fedyanin. Observation of hybrid state

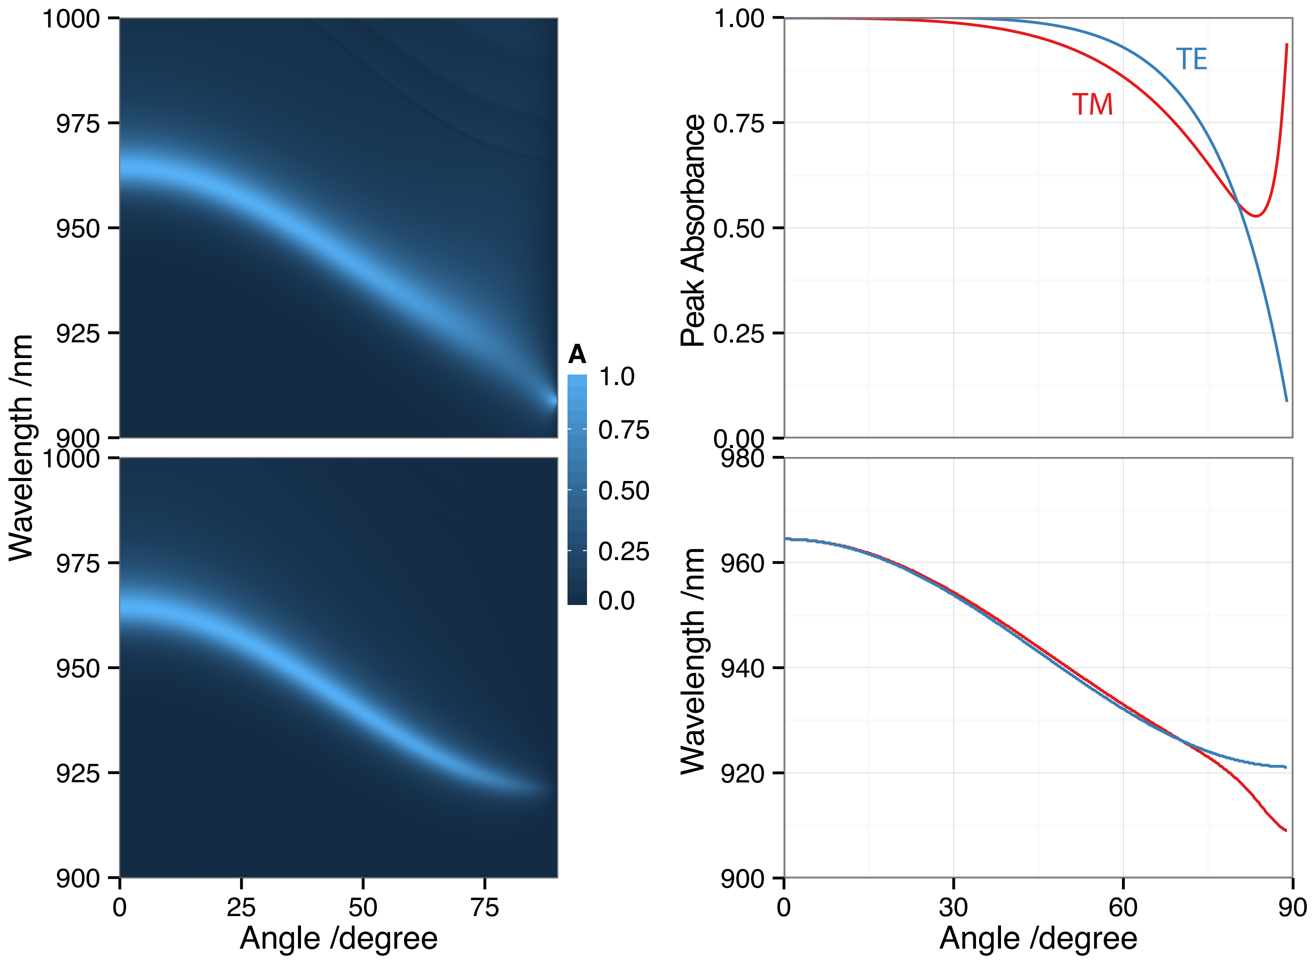


**Figure S5.** Angular dispersion of the Tamm mode, illuminated from the air-Au side. The structure is that of Fig. 4 (b) of the main manuscript, i.e. a thin Au film followed by a thick DBR of 50 pairs. The angle of incidence with respect to the normal is taken in air. Top and bottom panels correspond to TM- and TE-polarisation, respectively. The right panels trace the spectral position and maximum value of absorbance for the Tamm mode.


of Tamm and surface plasmon-polaritons in one-dimensional photonic crystals. *Applied Physics Letters*, 103(6):061112, 2013.

[5] Ritwick Das, Triranjita Srivastava, and Rajan Jha. Tamm-plasmon and surface-plasmon hybrid-mode based refractometry in photonic bandgap structures. *Opt. Lett.*, 39(4):896, February 2014.

[6] X.-L. Zhang, J.-F. Song, X.-B. Li, J. Feng, and H.-B. Sun. Optical Tamm states enhanced broad-band absorption of organic solar cells. *Applied Physics Letters*, 101(24), 2012.
